# Supplementary material for: Hierarchical Experimentalist Agents
Source: arXiv:2606.29315 source file (2026-10-09)
Supplement: Supplementary file 1 [file app_ablation.tex]

% ============================================================
%  APPENDIX — place inside your \appendix block
% ============================================================
 
\section{Prompt Ablation Study: Full Results}
\label{app:ablation}

Table~\ref{tab:ablation_legend} describes the four ablation levels and
the components removed at each step.

% --- Legend table -----------------------------------------
\begin{table}[h]
\centering
\small
\caption{%
  Ablation levels and the prompt components removed at each step.
  Removals are cumulative: each level also removes everything
  stripped at earlier levels.
}
\label{tab:ablation_legend}
\setlength{\tabcolsep}{6pt}
\begin{tabular}{clp{7cm}}
\toprule
\textbf{Level} & \textbf{Name} & \textbf{Component removed} \\
\midrule
Full
  & Full prompt
  & Nothing removed; all hints enabled. \\
\addlinespace[3pt]
Abl.\ 1
  & No strategy tips
  & Explicit tool-invocation order and collision-direction
    instructions (e.g.\ which side of the green ball to strike
    in order to push it toward the target). \\
\addlinespace[3pt]
Abl.\ 2
  & No physics rules
  & Remaining physics heuristics and placement guidelines
    (e.g.\ recommended horizontal offsets; side-of-green-ball
    placement rules for reliable lateral impulse). \\
\addlinespace[3pt]
Abl.\ 3
  & No tool feedback
  & Rich observation outputs: corrective offset messages on
    invalid placements (e.g. how much distance to move away from the overlapping object) \\
\addlinespace[3pt]
Abl.\ 4
  & No geometry tool
  & Level-specific analysis tool
    (\texttt{compute\_gap\_analysis} for \textit{Down to Earth};
    \texttt{compute\_relative\_positions} for
    \textit{Two Body Problem}). \\
\bottomrule
\end{tabular}
\end{table}
