# Supplementary material for: Hierarchical Experimentalist Agents
Source: arXiv:2606.29315 source file (2026-10-09)
Supplement: Supplementary file 2 [file app_HeXA.tex]

% ============================================================
%  Appendix: HExA
% ============================================================
\section{HExA: More Methodological Details}
\label{app:hexa}





\subsection{Overview}
\label{sec:overview}
 
Many agentic tasks require an LLM to go beyond its parametric knowledge and actively interact with an environment to gather the instance-specific information needed to complement existing parametric knowledge in complex queries or experimental tasks; or to fundamentally interact and experiment in an unseen domain to reason, act and correctly complete some novel user task or query beyond the model's existing parametric knowledge and capabilities.
An intuitive paradigm for learning in such settings and retaining useful reusable information is via inference-time in-context skill augmentation: distilling reusable strategies and common pitfalls from \textbf{\emph{interaction experience and active experimentation}} into compact natural-language \textbf{\emph{skills}} that are reusable in the agent's context at the start of each new episode, amortizing cost of exploration and skill reuse in newer tasks or domains.
Turning this idea into a working self-improving framework, however, faces three difficulties: (1) the agent has no access to oracle solutions, expert demonstrations, or optimal offline data from the task family; (2) there is no human or oracle guided skills to start with and no external reward model or verifier beyond the interaction feedback on the unseen domain to bootstrap the learning; and (3) the skill library must be autonomously evolved and remain compact and bounded to fit within the agent's context window while still capturing the most useful knowledge.

In our paper, we introduce \textbf{\textit{HExA}} (Hierarchical Experimentalist Agents), shown in Figure~\ref{fig:hexa_main}, a training-free, in-context reinforcement learning framework that autonomously discovers, evolves, and transfers reusable skills without parameter updates, external feedback, or human annotation.
At its core, HExA operates a two-agent loop over a sequence of rounds (\ref{sec:framework}): an \emph{actor} $\pi_{\mathrm{act}}$ actively experiments with the environment through a tool-call interface, generating trajectories of successes and failures; an \emph{evolver} $\pi_{\mathrm{ev}}$ reads batches of these trajectories, contrasts high-reward against low-reward episodes, and distills the result into an evolving external \emph{skill bank} $\mathcal{K}$ via a two-phase contrastive and failure-analytic distillation process (\ref{sec:distillation}).
A reward-weighted \emph{retriever} (\ref{sec:retrieval}) selects the most relevant skills and injects them into the actor's context before each subsequent episode, so that the cost of exploration is amortized across problem instances rather than paid from scratch each time.


A key risk in any iterative skill-evolution loop is \emph{skill drift}: the evolver may accumulate increasingly narrow strategies that overfit to the particular instances seen so far, while discarding general principles that would transfer to new instances.
To address this, HExA supports multiple initialisation and update regimes (\ref{sec:regimes}) that control the balance between retaining proven skills and incorporating new evidence, ranging from a frozen offline bank to a fully online evolution strategy.
Beyond within-task learning, HExA further enables \emph{cross-task skill transfer} (\ref{sec:transfer}): skill banks evolved on one or more source task families are re-grounded by the evolver onto a structurally related target task, enabling zero-shot transfer with no target-task interaction.
In this way, HExA autonomously constructs task-specific skills that can be deployed with any frozen LLM at inference time to enable in-context self-improvement without weight updates.







\subsection{Problem Formulation}
\label{sec:problem-formulation}

We consider a task family $\ell$ consisting of a set of task instances $\{(\ell, s_j)\}$, where each instance is identified by an index $s_j$ (e.g., a random seed) that determines the specific configuration of the environment (geometry, parameters, initial conditions).
The agent interacts with each instance through a tool-call interface exposing a set of tools $\mathcal{F}$, and the environment defines a binary success predicate $\textsc{Goal}_\ell$ that evaluates the outcome of a completed simulation.
 
At each iteration $t$ of an episode, the agent observes the conversation history $h_t = (o_0, a_1, o_1, \ldots, a_{t-1}, o_{t-1})$, where $o_i$ is an observation returned by a tool call and $a_i \in \mathcal{F}$ is a tool invocation, and selects the next action according to its policy $\pi$.
The episode terminates after at most $T$ iterations or when the agent issues a terminal action.
We define a success indicator $y_j$ for task instance $s_j$ as:
%
\begin{equation}
\label{eq:success}
y_j(\pi;\, \ell,\, \mathcal{G}) \;=\; \mathbb{I}\bigl[\textsc{Goal}_\ell\!\left(\textsc{Sim}(\tau_j)\right) = \text{true}\bigr], \qquad \tau_j \sim \pi(\cdot \mid \ell,\, s_j,\, \mathcal{G}),
\end{equation}
%
where $\tau_j$ is the trajectory generated by $\pi$, $\textsc{Sim}$ runs the environment simulation to completion, and $\mathcal{G}$ is an optional skill context.
 
Our goal is to maximize the solve rate across instances of $\ell$ without any parameter updates to $\pi$.
To this end, we introduce a natural-language \emph{skill bank} $\mathcal{K}$, a structured collection of reusable strategies and common-mistake records that is prepended to the agent's system prompt at the start of each episode:
%
\begin{equation}
\label{eq:skill-augmented}
\tau_j \sim \pi(\cdot \mid \ell,\, s_j,\, \mathcal{G}), \qquad \mathcal{G} = \textsc{Retriever}(\mathcal{K},\, \ell,\, M,\, N),
\end{equation}
%
where $\textsc{Retriever}$ selects the top-$M$ skills by reward and top-$N$ mistakes from $\mathcal{K}$.
The skill bank $\mathcal{K}$ is constructed and evolved entirely through HExA's actor-evolver loop (Section~\ref{sec:framework}), with no human annotation, external teacher, or access to oracle solutions.
Each trajectory is additionally assigned a scalar reward $r(\tau_j) \in [-1, +1]$ that reflects both outcome and efficiency (Eq.~\ref{eq:reward}), providing the evolver with a richer learning signal than the binary success indicator alone.

\subsection{The HExA Framework}
\label{sec:framework}


\begin{figure}[H]
  \centering
  \includegraphics[width=\linewidth]{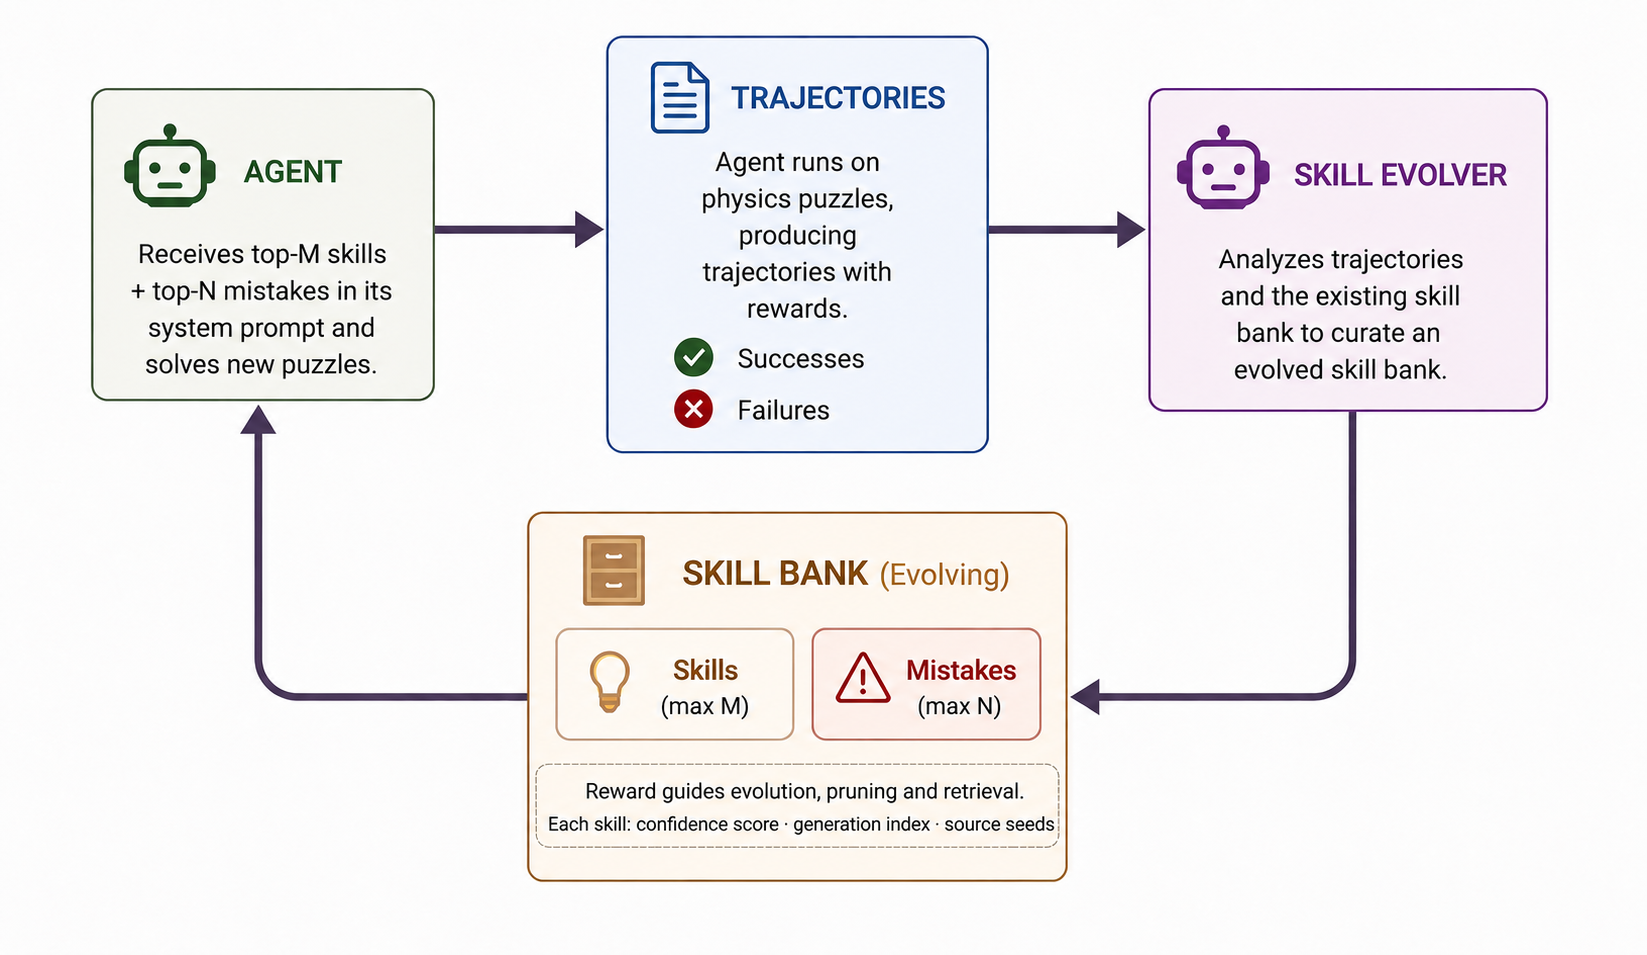}
  \caption{%
    \textbf{The \textsc{HExA} actor-evolver loop.}
    The actor receives distilled skills in its system prompt and runs on
    physics puzzles, producing trajectories annotated with rewards
    (successes~\cmark, failures~\xmark).
    The Skill Evolver analyzes these trajectories and curates the
    evolving Skill Bank: skills (max~M) are merged, pruned, or promoted
    by reward signal, and common mistakes (max~N) are updated accordingly.
    Each skill carries a generation index tracking its lineage across
    evolution rounds (Eq.~\ref{eq:confidence}).
    The updated bank is injected back into the actor's system prompt for
    the next round, closing the loop.
  }
  \label{fig:hexa_loop}
\end{figure}



\begin{figure}[h]
  \centering
  \begin{subfigure}[t]{0.48\linewidth}
    \centering
    \includegraphics[width=\linewidth]{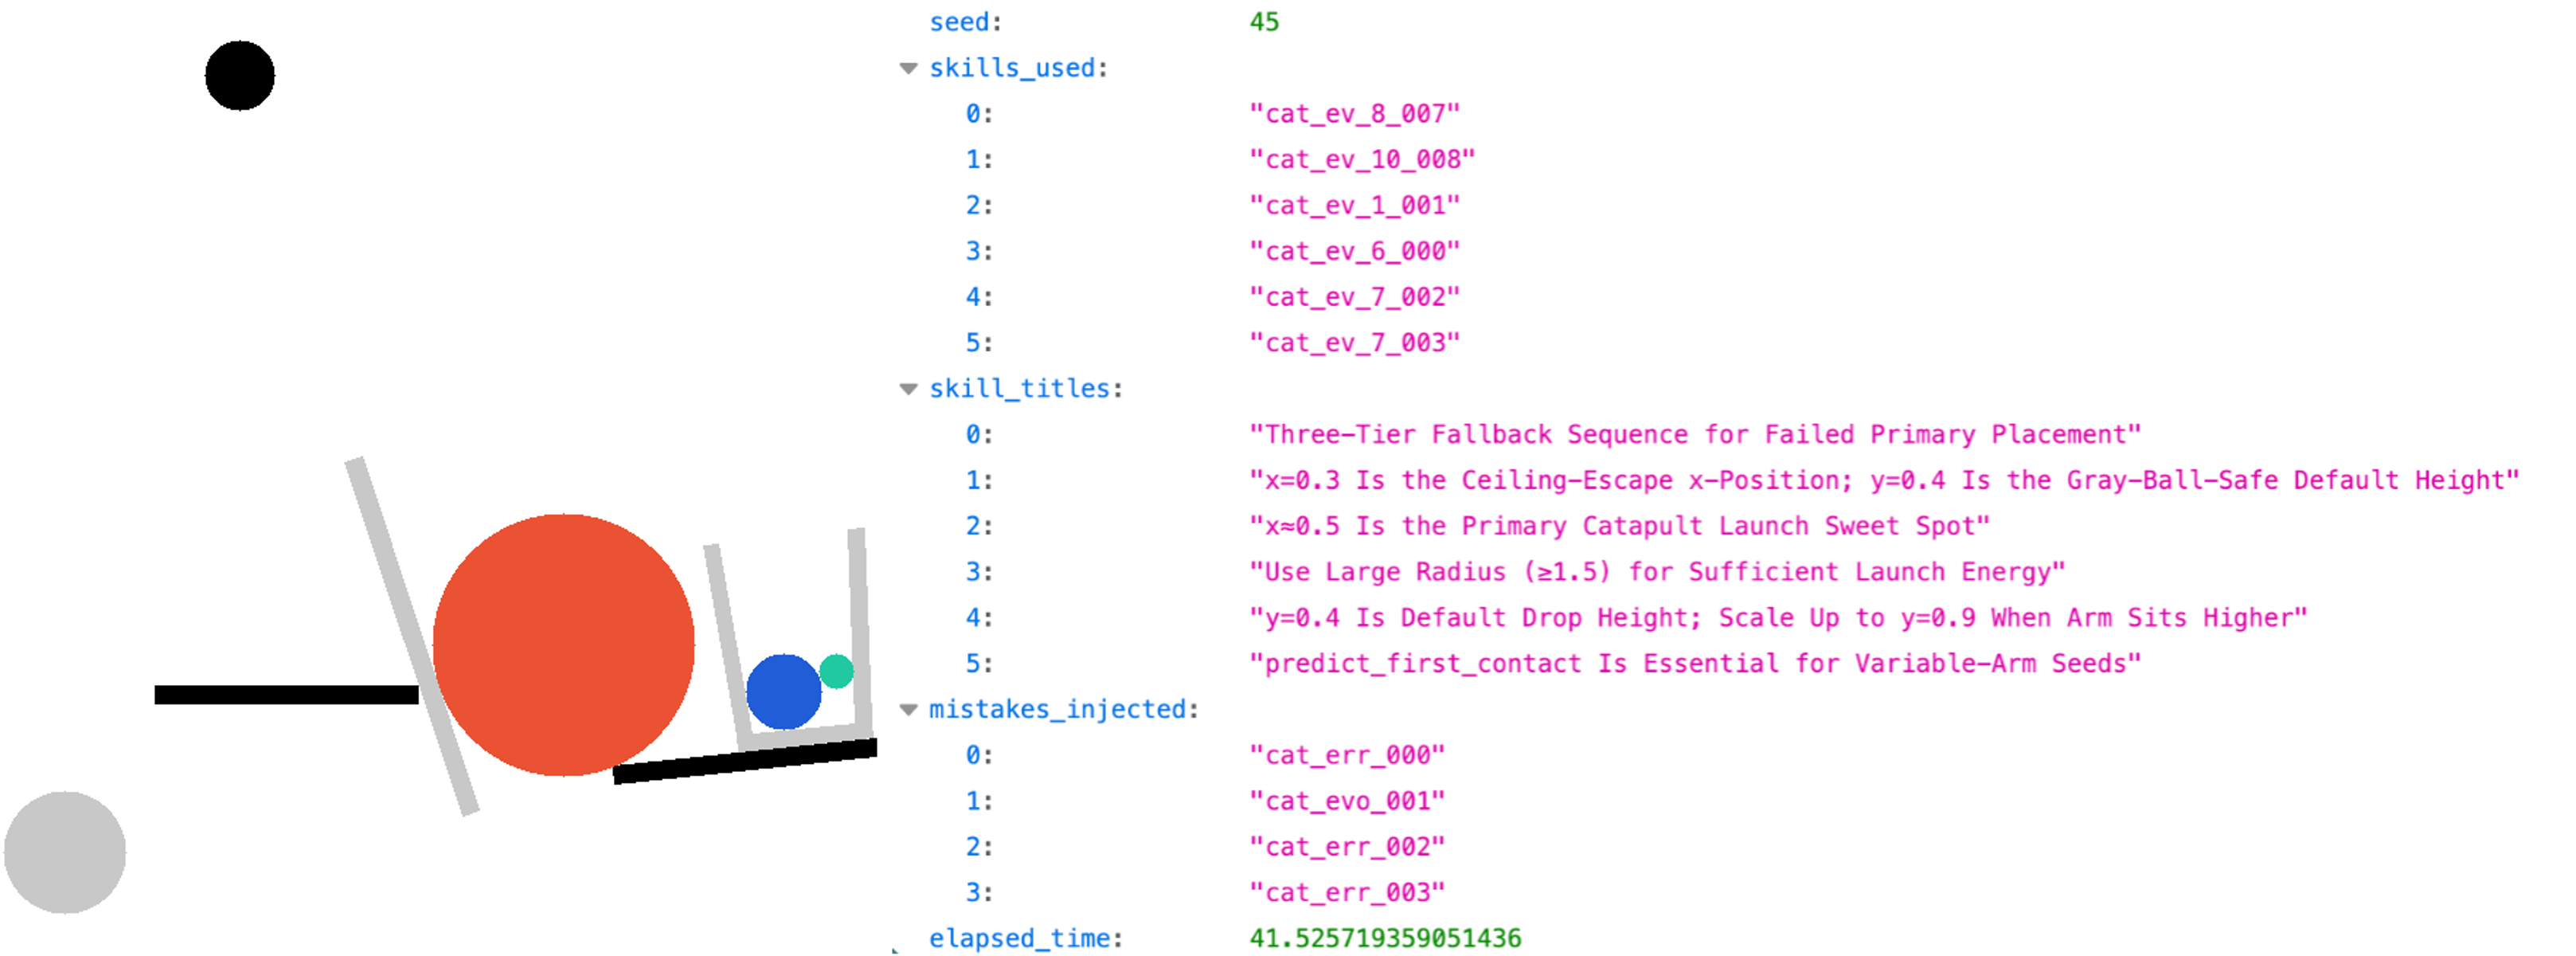}
    \caption{Example on \texttt{catapult} with its skill bank.}
    \label{fig:running_example}
  \end{subfigure}
  \hfill
  \begin{subfigure}[t]{0.48\linewidth}
    \centering
    \includegraphics[width=\linewidth]{figures/Feedback_Loop.png}
    \caption{\textsc{HExA} actor--evolver--retriever loop.}
    \label{fig:hexa_loop2}
  \end{subfigure}
  \caption{%
    \textbf{\textsc{HExA} learns reusable skills through an actor--evolver--retriever loop.}
    \textbf{(a)}An example on \texttt{catapult} level illustrates the kind of physics reasoning skills \textsc{HExA} distills.
    \textbf{(b)} In each round, the actor generates reward-tagged trajectories, the evolver
    updates the skill bank, and the retriever injects the most relevant skills back into the
    actor for the next attempt.
  }
  \label{fig:hexa_overview_main}
\end{figure}


HExA instantiates the skill-augmented policy of Eq.~\ref{eq:skill-augmented} through a two-agent architecture operating over a sequence of \emph{rounds}.
An \textbf{actor} $\pi_{\mathrm{act}}$ (any tool-augmented LLM) generates trajectories by interacting with the environment, while an \textbf{evolver} $\pi_{\mathrm{ev}}$ (which may be the same model) reads batches of actor trajectories and distills them into the skill bank $\mathcal{K}$.
At the start of each new episode, the $\textsc{Retriever}$ selects the most relevant skills from $\mathcal{K}$ and injects them into the actor's context, so that each subsequent trajectory benefits from the accumulated experience of all prior ones.
 
This loop can be viewed as an instantiation of in-context reinforcement learning~\citep{laskin2022context,moeini2025survey}: the agent's policy improves over rounds through context augmentation rather than weight updates, and the skill bank serves as a compressed, curated form of the cross-episode context that classical in-context RL methods maintain in raw form.
Unlike standard in-context RL, however, HExA does not require pretraining on a task distribution; it operates on a single frozen model and learns from scratch on each task family.







\subsubsection{Trajectory Reward}
\label{sec:reward}

Not all trajectories are equally informative. A fast, decisive solve reveals a high-reward strategy; a failure that explored extensively yields richer material for the evolver than one that abandoned the episode after a single attempt.
To communicate this signal, we assign a scalar reward $r(\tau) \in [-1, +1]$ to each trajectory $\tau$, reflecting both \emph{outcome} (success or failure) and \emph{efficiency} (iteration count $t$ at termination):
%
\begin{equation}
r(\tau) \;=\;
\begin{cases}
+1.00 & \text{success},\; t \le 3 \\
+0.75 & \text{success},\; t \le 7 \\
+0.50 & \text{success},\; t \le 15 \\
+0.25 & \text{success},\; t \le T \\[3pt]
-0.50 & \text{failure},\; t \ge 10 \\
-0.75 & \text{failure},\; t < 10
\end{cases}
\label{eq:reward}
\end{equation}
%
The asymmetry in failure penalties is deliberate: an agent that explores extensively before failing produces richer interaction records for the evolver to extract partial skills and diagnose mistakes.
 



\begin{algorithm}[h]
\caption{HExA}
\label{alg:HeXa_algo_app}
\DontPrintSemicolon
\KwIn{Base agent $\pi_{\text{act}}$, evolver $\pi_{\text{ev}}$, level $\ell$,
      regime $\mathcal{R} \in \{\text{Offline}, \text{Off2On}, \text{Online}\}$,
      update strategy $\mathcal{U} \in \{\text{Evolution}, \text{Iterative}, \text{None}\}$,
      rounds $R$, trajectories per round $x$, initial batch size $N_0$,
      retrieval sizes $M, N$}
\KwOut{Final skill bank $\mathcal{K}_R$ and per-round trajectories $\{\mathcal{T}^{(n)}\}_{n=1}^{R}$}

\tcp{Stage 1: Initialise skill bank $\mathcal{K}_0$}
\uIf{$\mathcal{R} \in \{\text{Offline},\ \text{Off2On}\}$}{
    Collect batch $\mathcal{T}_0$ of $N_0$ trajectories from $\pi_{\text{act}}$ on $\ell$\;
    $\mathcal{K}_0 \gets \text{Evolver}(\emptyset, \mathcal{T}_0)$ \tcp*{teacher-driven distillation}
}
\Else{
    $\mathcal{K}_0 \gets \emptyset$ \tcp*{cold start (Online)}
}

\BlankLine
\tcp{Stage 2: Iterative rounds of generation, distillation, and update}
\For{$n = 1, 2, \dots, R$}{
    $\mathcal{G}_n \gets \text{Retriever}(\mathcal{K}_{n-1}, \ell, M, N)$ \tcp*{retrieve top-$M$ skills, top-$N$ mistakes}
    $\mathcal{T}^{(n)} \gets \emptyset$\;
    \For{$i = 1, \dots, x$}{
        $\tau_i \gets \pi_{\text{act}}(\ell \mid \mathcal{G}_n)$ \tcp*{run skill-augmented agent}
        $r(\tau_i) \gets \textsc{Reward}(\tau_i)$ \tcp*{Eq.~\ref{eq:reward}}
        $\mathcal{T}^{(n)} \gets \mathcal{T}^{(n)} \cup \{(\tau_i, r(\tau_i))\}$\;
    }
    \uIf{$\mathcal{R} = \text{Offline}$}{
        $\mathcal{K}_n \gets \mathcal{K}_{n-1}$ \tcp*{frozen bank}
    }
    \uElseIf{$\mathcal{U} = \text{Evolution}$}{
        $\mathcal{K}_n \gets \text{Evolver}(\mathcal{K}_{n-1}, \mathcal{T}^{(n)})$ \tcp*{merge, revise, prune}
    }
    \ElseIf{$\mathcal{U} = \text{Iterative}$}{
        $\mathcal{K}_n \gets \text{Evolver}(\emptyset, \mathcal{T}^{(n)})$ \tcp*{re-distil from new trajectories only}
    }
}
\KwRet{$\mathcal{K}_R,\ \{\mathcal{T}^{(n)}\}_{n=1}^{R}$}
\end{algorithm}



\subsubsection{Skill Distillation from Experimentation on Self-Proposed Hypotheses}
\label{sec:distillation}


At each round $n$, the evolver $\pi_{\mathrm{ev}}$ receives the batch of trajectories $\mathcal{T}^{(n)} = \mathcal{T}^{(n),+} \cup \mathcal{T}^{(n),-}$ generated by the actor, where $\mathcal{T}^{(n),+}$ and $\mathcal{T}^{(n),-}$ denote the successful and failed subsets respectively, each annotated with its scalar reward.
The evolver performs a two-phase distillation to extract complementary forms of knowledge.
 
\paragraph{Phase 1: Contrastive skill extraction.}
Given the full batch $\mathcal{T}^{(n)}$ with reward annotations, the evolver contrasts high-reward trajectories against low-reward ones to identify the strategies and insights that distinguish success from failure.
This produces 4--6 \emph{strategy skills}, each consisting of a short title, a 2--3 sentence natural-language principle describing the underlying mechanism, and an applicability predicate specifying when the skill is relevant.
The evolver is instructed to weight its analysis by reward: skills derived from fast, efficient solves are treated as more reliable than those from trajectories that barely succeeded.
 
\paragraph{Phase 2: Mistake and partial-skill extraction.}
Focusing on the failure subset $\mathcal{T}^{(n),-}$, the evolver produces two complementary outputs.
\emph{Common mistakes} are structured records $\mu = (\delta, \rho, \alpha)$, where $\delta$ describes the error, $\rho$ identifies its root cause (the broken causal belief that led to it), and $\alpha$ specifies a concrete corrective strategy.
\emph{Partial skills} capture correct reasoning steps that appeared \emph{within} otherwise failed trajectories: an agent may have identified a valid strategy or correctly diagnosed a mechanism before making an error elsewhere.
These partial successes cannot be discovered from successful trajectories alone and are a distinctive source of learning signal in HExA.


 


\subsubsection{Skill Bank}
\label{sec:skillbank}

Distilled knowledge is stored in the skill bank $\mathcal{K}$ with two collections, both indexed by task family: a set of \emph{skills} (reusable strategy and principles) and a set of \emph{mistakes} (patterns recording and describing recurring failure modes to avoid).
Each skill carries a reward label, computed from the interaction rewards of the trajectories that demonstrated it:
%
\begin{equation}
r_k \;=\; \operatorname{clamp}\!\left(\frac{\bar{r}_{\mathrm{src}} + 1}{2},\; 0.1,\; 1.0\right),
\label{eq:confidence}
\end{equation}
%
where $\bar{r}_{\mathrm{src}}$ is the mean reward of the source trajectories from which the skill was extracted.
Skills derived from fast, efficient solves carry higher rewards; skills surfaced from partial reasoning within failed trajectories carry lower rewards but may still encode valuable discoveries.
The skill bank is hard-capped at $M_{\max}$ skills and $N_{\max}$ mistakes per task family to prevent the injected context from growing without bound and to force the evolver to prioritize the most informative knowledge during evolution rounds. This is where the reward labels and the creation of hierarchical skills, help in improving the skill bank even though it is capped at a maximum number of skills.
 





\subsubsection{Skill Retrieval and Injection}
\label{sec:retrieval}

At the start of each episode, the $\textsc{Retriever}$ selects the top-$M$ skills from $\mathcal{K}$ sorted by reward $r_k$ and the top-$N$ mistakes for the relevant task family, and injects them into the actor's system prompt as the structured skill context $\mathcal{G}$ defined in Eq.~\ref{eq:skill-augmented}.
The actor receives this block alongside the standard task description and tool documentation, and is free to use or disregard individual skills based on its own reasoning about the current instance.
This injection mechanism is deliberately simple: it adds a fixed-size prefix to the prompt rather than modifying the agent's architecture or decoding procedure, making HExA compatible with any tool-augmented LLM, including closed-source API-served models.







\subsubsection{Initialisation, Update Regimes, and Full Algorithm}
\label{sec:regimes}


The loop described above admits several configurations that vary along two orthogonal axes:
how the skill bank is \emph{initialised} before evaluation begins, and how it is
\emph{updated} between rounds.
Algorithm~\ref{alg:HeXa_algo_app} summarizes the full procedure; we now describe the design axes it parameterizes.


\paragraph{Initialisation.}
In the \textbf{Offline} and \textbf{Offline-to-Online} (Off2On) regimes, a warm-start batch of $N_0$ trajectories is collected from the base actor (without any skill context) and distilled into an initial bank $\mathcal{K}_0$ via $\text{Evolver}(\emptyset, \mathcal{T}_0)$ (Algorithm~\ref{alg:HeXa_algo_app}, lines~3--4). In the \textbf{Pure Online} regime, the bank starts empty ($\mathcal{K}_0 = \emptyset$) and the agent must bootstrap skills entirely from its own online interactions (line~6).
 
\paragraph{Update strategy.}
Given trajectories from round $n$, the bank can be updated in two ways.
Under \textbf{Evolution}, the evolver receives both the current bank and the new trajectories, producing $\mathcal{K}_n = \text{Evolver}(\mathcal{K}_{n-1}, \mathcal{T}^{(n)})$ by merging, revising, or pruning existing skills in light of new evidence (line~17).
Under \textbf{Iterative Replacement}, the evolver distills $\mathcal{K}_n = \text{Evolver}(\emptyset, \mathcal{T}^{(n)})$ purely from the new trajectories, discarding all prior skills (line~19).
In the Offline regime, the bank is frozen after initialisation ($\mathcal{K}_n = \mathcal{K}_{n-1}$, line~15).









 
Crossing these axes yields five concrete variants: Offline (static bank), Off2On with Evolution, Off2On with Iterative Replacement, Pure Online with Evolution, and Pure Online with Iterative Replacement.
We compare these empirically in \ref{sec:experiments}.


Finally we see that the Off2On~+~Evolution variant works best across all settings and is thus the variant that we generally refer to as HExA in the rest of the paper.




\subsection{Cross-Task Skill Transfer}
\label{sec:transfer}
 
The skill banks produced by HExA encode task-family-specific strategies, but the underlying principles are often more general: momentum conservation, lever mechanics, collision geometry, and similar structural insights recur across task families that share physical or procedural primitives.
HExA exploits this by synthesizing a \emph{cross-task skill bank} for a target task family from the evolved banks of one or more source families, with no target-task trajectories required.
 
Given source banks $\mathcal{K}_{\ell_1}, \ldots, \mathcal{K}_{\ell_S}$ and a textual description of the target task family $\ell^*$, the evolver receives all source skills together with the target description and is prompted to:
%
\begin{enumerate}[leftmargin=1.5em,itemsep=2pt]
\item identify which source skills encode principles that are structurally relevant to the target (based on shared physical or procedural primitives),
\item re-ground each selected principle in the entities and mechanics of the target scene, and
\item calibrate reward based on how directly the principle transfers (skills corroborated by multiple source banks receive higher reward).
\end{enumerate}
%
The synthesised bank $\mathcal{K}_{\ell^*}$ is then injected into the actor's context via the same $\textsc{Retriever}$ mechanism as within-task skills.
This enables zero-shot transfer: the actor attempts the target task with the benefit of cross-task skills but without having seen any target-task trajectories.
 
Importantly, cross-task transfer and within-task skill evolution are complementary.
The synthesised bank can serve as the initialisation $\mathcal{K}_0$ for a subsequent within-task HExA run, combining the benefits of transferred knowledge with task-specific refinement.





\subsection{Design Principles}
\label{sec:design-principles}
 
Several design choices in HExA merit explicit discussion.
 
\paragraph{Domain agnosticism.}
Nothing in the framework above assumes a particular domain.
The actor interacts with the environment through a generic tool-call interface; the evolver reads trajectory text and produces structured JSON.
The only domain-specific components are the tool suite exposed by the environment and the system prompt describing the task, both of which are inputs to HExA rather than parts of its architecture.
We instantiate and evaluate HExA on physics puzzles in \S\ref{sec:experiments}, but the same framework applies to any setting where an agent must learn from sequential interactions with an environment.

\paragraph{Reward Function Agnostic.}
As we have shown previously in our experiments, rewards from environment interactions and shaped according to the needs of the user help HExA more. But the evolver can guide skill creation and learning even without it. So this reward agnostic nature of HExA make it widely applicable in domains where even environment reward might not be present. Moreover in cases where there is presence of such rewards and additional feedback, we can plug in any reward function to further guide skill acquisition either guided by users or designed by the LLM evolver itself.
 
\paragraph{No weight updates.}
HExA is entirely in-context: neither the actor nor the evolver undergoes any parameter updates.
All adaptation occurs through the evolving skill bank, which modifies the actor's behavior by changing the textual context it conditions on.
This makes HExA compatible with closed-source, API-served models and avoids the computational cost and catastrophic-forgetting risks of fine-tuning.
 
\paragraph{Hierarchical skill structure.}
The skills in $\mathcal{K}$ are hierarchical in two senses.
First, they abstract over low-level actions (specific tool calls and parameter values) into high-level strategy descriptions, compressing lengthy trajectories into concise principles.
Second, skills are learned iteratively while the agent has access to previously distilled skills, so later skills implicitly build on earlier ones.
The evolver may revise a skill in light of new evidence or merge two complementary skills into a more general one, producing a form of meta-learning: the agent learns not just strategies but \emph{how to learn strategies} from interactions.
 
