# Supplementary material for: Hierarchical Experimentalist Agents
Source: arXiv:2606.29315 source file (2026-10-09)
Supplement: Supplementary file 3 [file app_results_final.tex]

\section{Additional Experimental and Result Details}
\label{app:exp_res_final}

\input{tables/interphyre_main}
 
\input{tables/reward_ablation_main}

\input{tables/variants_compact}

\input{tables/external_compact}
\input{tables/transfer_merged}






\subsection{Instantiation of HExA}
\label{app:exp_res_final_instantiation}

\textsc{HExA} is also flexible enough to ingest additional experimental evidence
such as trajectory rewards, which are a function of outcome reward and efficiency
(Appendix~\ref{sec:reward}), to further guide skill evolution and retrieval. The
skill reward label $r_k$ is in turn a function of the trajectory rewards of the
trajectories that invoked the skill,
\begin{equation}
\label{eq:weight}
r_k = \operatorname{clamp}\!\left(\frac{\bar{r}_{\mathrm{src}}+1}{2},\,0.1,\,1.0\right),
\end{equation}
where $\bar{r}_{\mathrm{src}}$ is the mean reward of those source trajectories.
Depending on experimental settings, users can define any trajectory reward and skill reward; HExA as a framework is agnostic of these choices. We also tried skill evolution without rewards, using the evolver LLM's prior knowledge itself to guide skill bank update, ignoring the useful environment grounded rewards. Our ablations in Table~\ref{tab:ablations}c show that reward labeled skill banks perform the best. Thus, our default experimental setting for \textsc{HExA} is Off2On~+~Evolution with reward labeled skills.





\subsection{HExA on Interphyre Details}



\paragraph{Does active experimentation and skill creation help agents solve complex tasks?}
On levels where a single \textsc{ReAct} trajectory fails, we test whether
distilling interaction traces into an evolving skill bank improves over both
baselines that accumulate no reusable skills (\textsc{Zero-shot}, \textsc{ReAct},
Reflexion) and external-memory baselines that retain past episodes rather than
distilling them (Episodic RAG, MemRL). On the two hardest levels, where the base
Claude Sonnet model makes little or no progress, \textsc{HExA} reaches
$82.7\pm11.4\%$ on \texttt{catapult} and $96.0\%$ on
\texttt{pass\_the\_parcel}, compared with $0.0\%$/$0.0\%$ for
\textsc{Zero-shot}, $11.0\pm3.0\%$/$20.0\%$ for \textsc{ReAct},
$21.3\pm2.5\%$/$32.0\%$ for Reflexion, $60.8\%$/$60.0\%$ for
Episodic RAG, and $33.3\%$/$46.0\%$ for MemRL
(Table~\ref{tab:interphyre}). Figure~\ref{fig:catapult45_simframes} shows a
representative \texttt{catapult} seed where retrieved skills guide
\textsc{HExA} to a solution in a handful of interactions while \textsc{ReAct}
exhausts its budget.

The pattern also holds for weaker open-weight models. On
\texttt{down\_to\_earth}, \textsc{HExA} raises Qwen-2.5-7B from
$63.3\pm3.4\%$ to $82.7\pm5.2\%$ and Qwen-2.5-3B from
$8.3\pm0.9\%$ to $23.3\pm0.9\%$; on
\texttt{two\_body\_problem}, it raises them from $12.0\%$ to
$50.0\pm3.3\%$ and from $7.3\pm0.9\%$ to $12.0\%$, respectively.
Storing experience alone is not sufficient: on \texttt{down\_to\_earth} with
Qwen-2.5-7B, Episodic RAG and MemRL reach $42.7\%$ and $36.0\%$,
respectively, below memoryless \textsc{ReAct} at $63.3\%$. Reflexion reaches
$76.0\%$ there, but requires a second trial on each seed. These comparisons
indicate that the improvement comes from distilling prior interactions into
reusable strategies rather than from additional retries or merely including past
experience in the prompt.


\paragraph{Can \textsc{HExA} leverage learned skills for more efficient
exploration and experimentation?}
Spending more compute on interaction does not by itself raise task success, so we
record average turns per seed as an efficiency proxy alongside solve rate
(Figure~\ref{fig:cum_iter_both}, Table~\ref{tab:catapult_cost}).
Accuracy and cost move together: \textsc{HExA} lowers the average from $22.9$
turns under \textsc{ReAct} to $12.5\pm0.9$ on \texttt{catapult}, roughly
$45\%$ fewer, and from $18.7$ to $5.8$ on \texttt{pass\_the\_parcel}.
Thus, the additional successes require less interaction per instance rather than
more.

\textsc{HExA} is also the cheapest persistent memory to carry, injecting
$2{,}392$ tokens per episode on \texttt{catapult}, compared with $6{,}706$
for Episodic RAG and $8{,}135$ for MemRL
(Table~\ref{tab:interphyre}). The skill bank has fixed capacity, whereas storing
rollouts scales with the rollout cap rather than with the distilled knowledge.
Converting past experience into a reusable skill bank therefore amortizes the
cost of future experimentation instead of re-paying it each episode.

Figures~\ref{fig:build_then_freeze} and~\ref{fig:astra_catapult} trace the
protocol end to end on \texttt{catapult}: the bank accumulates over the training
seeds, is then frozen, and is evaluated against the same baselines on disjoint
held-out seeds for Claude Sonnet and GPT-6-Astra. The ordering established during
bank construction persists after freezing, while the stronger GPT-6-Astra actor
requires fewer rounds to acquire the useful skills.


\paragraph{How does in-context skill learning compare with gradient-based adaptation?}
The advantage also appears against a weight-update baseline. At a matched
50-unique-seed budget, GRPO fine-tuning Qwen-2.5-3B reaches $20\%$ on
\texttt{down\_to\_earth} and $6\%$ on
\texttt{two\_body\_problem}, compared with \textsc{HExA}'s $23.3\%$ and
$12.0\%$, respectively (Appendix~\ref{app:results:grpo}). Skills distilled
from early trajectories become immediately available to subsequent episodes
through context, whereas gradient-based adaptation must accumulate rollout signal
before the same information is encoded in model weights. With additional training,
GRPO eventually closes or reverses this low-data gap; complete training curves
and settings are reported in Appendix~\ref{app:results:grpo}.


\paragraph{Which ingredients drive improvements in \textsc{HExA}?}
Using the instantiation axes defined in Section~\ref{sec:instantiation}, we study
how each one aids learning from experimentation.



\paragraph{Can \textsc{HExA} leverage learned skills for more efficient
exploration and experimentation?}
Spending more compute on interaction does not by itself raise task success, so we
record the average number of turns per seed as an efficiency proxy alongside
solve rate (Figure~\ref{fig:cum_iter_both}, Table~\ref{tab:catapult_cost}).
Accuracy and cost move together: \textsc{HExA} lowers the average from $22.9$
turns under \textsc{ReAct} to $12.5 \pm 0.9$ on \texttt{catapult}, roughly $45\%$
fewer, and to $5.8$ from $18.7$ on \texttt{pass\_the\_parcel}, so the extra
successes come with less computation per instance rather than more. It is also
the cheapest memory to carry, at $2{,}392$ injected tokens per episode against
$6{,}706$ and $8{,}135$ for the episodic baselines
(Table~\ref{tab:interphyre}); the bank is a fixed size, so its cost is constant
in the number of episodes played, whereas storing rollouts scales with the
rollout cap rather than with anything learned. Converting past experience into a
reusable skill bank therefore amortizes the cost of future experimentation
instead of re-paying it each episode.
\paragraph{Which ingredients drive improvements in \textsc{HExA}?}
Using the instantiation axes defined in Section~\ref{sec:instantiation}, we study
how each one aids learning from experimentation.





\subsection{Detailed Results of HExA on Other Benchmarks and Tasks}


\label{app:results:external}

\paragraph{Do the gains from experimentation and skill reuse hold beyond
\textsc{InterPhyre}?}
We repeat the same frozen-bank protocol on three external benchmark families:
interactive games, reasoning and planning, and open-ended scientific discovery,
against the same non-experimental and external-memory baselines.
Figure~\ref{fig:external_bench} summarizes each family as one score per actor,
averaged over that family's environments; Table~\ref{tab:external} reports the
per-task values. Token budgets, per-episode breakdowns, and exact paired tests are
reported in Appendices~\ref{app:results:external}--\ref{app:results:discovery}.

Across all four actor groups, \textsc{HExA} is the highest-performing memory
method. Neither episodic baseline is consistently beneficial:
\textsc{Episodic RAG} falls below no memory on the interactive games with
\texttt{gpt-oss-120b}, while \textsc{MemRL} falls below no memory on
\textsc{DiscoverPhysics}. Thus, each episodic-memory method imposes a cost in at
least one family, whereas the distilled bank improves every reported actor group.


\paragraph{Do distilled skills help when each instance is replayed?}
For the interactive games, each instance is played for three episodes with the
hidden task held fixed. Figure~\ref{fig:external_bench} reports \texttt{any},
the fraction of instances solved in at least one of the three episodes; the full
results additionally report \emph{ep3}, success on the final episode, which
measures how much the agent carries from its earlier attempts on the same instance.

The bank improves both actors and is also the cheapest persistent memory.
On Mastermind, \textsc{HExA} injects $971$ tokens per episode compared with
$1{,}957$ for Episodic RAG and $3{,}416$ for \textsc{MemRL}; on Maze, the
corresponding costs are $429$, $5{,}457$, and $7{,}027$ tokens.
Thus, the episodic baselines inject between $3.5\times$ and $16\times$ as much
context as the skill bank in these settings.

Storing episodes verbatim does not consistently transfer across instances:
a retrieved transcript from a previous instance can displace the actor's own
cross-episode observations rather than supplement them with a reusable abstraction.
\textsc{MemRL} is statistically indistinguishable from no memory in all three
settings in which it was run. In contrast, \textsc{HExA} compresses prior
experience into a much smaller set of strategies that can be reused across
instances while leaving more context available for the current interaction.


\paragraph{Do distilled skills help on reasoning and planning tasks?}
Every method receives the same rollout budget, so the comparison differs only in
what information is carried between items. \textsc{HExA} improves the frozen actor
on all four tasks, raising mean accuracy from $0.518$ with no memory to $0.744$,
and is the only memory method that improves every task rather than trading gains
on one task against losses on another.

Episodic RAG and \textsc{MemRL} reach mean accuracies of $0.606$ and $0.556$,
respectively. Storing previous rollouts therefore recovers part of the benefit,
but not most of it, despite the equal rollout budget. The additional gain from
\textsc{HExA} comes from making distilled strategies immediately available to
later items through context rather than carrying the original trajectories
themselves.


\paragraph{Do distilled skills help when the task is open-ended scientific discovery?}
On \textsc{DiscoverPhysics}, the skill bank contains experimentation strategies
rather than task solutions. This produces the largest aggregate margin among the
three external families: the judge's explanation score rises from $0.540$ with
no memory to $0.873$ with \textsc{HExA}.

The improvement also appears under the benchmark's strict success criterion.
On \texttt{oscillator}, pass rate at the $0.90$ explanation-score gate rises from
$0/15$ to $11/15$, whereas the baseline never clears the gate. On
\texttt{circle}, the benchmark reward alone does not improve significantly.
This is not inconsistent with the explanation-score gain: the evaluator
re-optimizes the submitted parameters against the agent's own trajectories, so
an incorrect functional form can still fit the observed data well. The explanation
metric therefore exposes improvements in discovering the underlying law that the
fit-based reward may not fully reflect.



%%%%%%%%%%%%% UTSAV Version %%%%%%%%%%%%%%%



\paragraph{Do the gains from experimentation and skill reuse hold beyond
\textsc{InterPhyre}?}
We repeat the same frozen-bank protocol on three external families --- interactive
games, reasoning and planning, and open-ended scientific discovery --- against the
same non-experimental and external-memory baselines.
Figure~\ref{fig:external_bench} reports each family as one score per actor,
averaged over that family's environments; the per-environment rows it averages,
the token budgets and the exact paired tests are in
Appendices~\ref{app:results:external}--\ref{app:results:discovery}.
\textsc{HExA} is the highest bar in all four actor groups. Neither episodic
baseline manages that: \textsc{Episodic RAG} sits below no memory on the games
with \texttt{gpt-oss-120b} and \textsc{MemRL} sits below it on
\textsc{DiscoverPhysics}, so each of them costs the actor something on at least
one family while the distilled bank costs it nothing on any.

\emph{Do distilled skills help when each instance is replayed?} On the two
interactive games every instance is played for three episodes with the hidden
task held fixed, so the panel reports \texttt{any}, success on at least one of
the three; the appendix additionally reports \emph{ep3}, success on the last
episode, which measures how much an agent has learned from its own earlier
attempts on that instance. The bank lifts both actors, and it is the cheapest
memory of the three by an order of magnitude: $971$ injected tokens against
$1{,}957$ for \textsc{Episodic RAG} and $3{,}416$ for \textsc{MemRL} on
Mastermind, and $429$ against $5{,}457$ and $7{,}027$ on Maze. Storing episodes
verbatim does not transfer across instances --- a prior instance's transcript
displaces the agent's own cross-episode observations rather than supplementing
them --- and \textsc{MemRL} is statistically indistinguishable from no memory in
all three settings it was run in, while injecting between $3.5$ and $16\times$ as
many tokens as the bank.

\emph{Do they help on reasoning and planning tasks?} Every arm here is given the
same rollout budget as \textsc{HExA}, so the only difference is what each one
carries between items. The bank improves the frozen model on all four tasks,
raising the mean from $0.518$ to $0.744$, and it is the only arm that improves
every task rather than trading one against another. Both episodic baselines land
between the two, at $0.606$ and $0.556$: storing the rollouts themselves recovers
part of the gain but not most of it, even at an equal budget. What helps is the
distilled strategy, which is available to later items immediately through
context.

\emph{Do they help when the task is open-ended discovery rather than a known
goal?} On \textsc{DiscoverPhysics} the bank holds experimentation strategies
rather than solutions, and it is the widest margin of the three families,
$0.540$ to $0.873$ on the judge's explanation score. The gain is not a graded
one: pass-rate at the strict $0.90$ gate goes from $0/15$ to $11/15$ on
\texttt{oscillator}, a gate the baseline never once clears. On \texttt{circle}
reward alone does not move significantly, which is informative rather than
inconsistent: that world's evaluator re-optimises the declared parameters against
the agent's own trajectories, so a wrong functional form can still fit the data
well.




\subsection{Instantiation and Ablations}



\emph{Does skill bank initialization and update matter?} We test three initializations---\emph{Offline},
\emph{Offline-to-Online} (\emph{Off2On}), and \emph{Online}. Both Offline and
Off2On warm-start the bank from $N_0$ base-actor trajectories collected with no
skill context, distilled into a fixed skill bank
$\mathcal{K}_0=\pi_{\mathrm{ev}}(\emptyset,\mathcal{T}_0)$; Offline then freezes
the bank, whereas Off2On keeps updating it after new rollouts. Online instead
starts empty ($\mathcal{K}_0=\emptyset$) and bootstraps skills purely from the
agent's own interactions. For updates we use two strategies---\emph{Evolving} and
\emph{Iterative Replacement}. In Evolving, we pass the evolver both the current
bank and the new round's trajectories, adding, merging, revising, or pruning
skills in light of this new evidence
($\mathcal{K}_n=\pi_{\mathrm{ev}}(\mathcal{K}_{n-1},\mathcal{T}^{(n)})$).
\emph{Iterative Replacement} instead rebuilds the bank from the current rollouts
alone ($\mathcal{K}_n=\pi_{\mathrm{ev}}(\emptyset,\mathcal{T}^{(n)})$), since in
the in-context RL loop the actor has already ingested prior skills, so the new
skills carry their influence plus the novelty of the latest rollouts. We thus
have five variants of skill bank initialization and update---\textit{Off2On} or
\textit{Online} initialization $\times$ \textit{Evolution} or \textit{Iterative
Replacement} update---plus the frozen Offline bank
($\mathcal{K}_n=\mathcal{K}_{n-1}$). We ablate these settings in
Table~\ref{tab:variants_compact} and Figure~\ref{fig:training_curves}, \emph{Off2On~+~Evolution} clearly performs the best, which is the default setting for HExA in all our final experimental results.
% reaching $84.0\%$ on \texttt{catapult} and $68.0\%$ on \texttt{pass\_the\_parcel}
% against $44.0\%$ and $58.0\%$ for a pure Online start and $56.0\%$ and $48.0\%$
% for Iterative Replacement.
\setlength{\intextsep}{0pt}
\setlength{\columnsep}{10pt}
\begin{wrapfigure}[24]{r}{0.48\linewidth}
  \vspace{-\intextsep}
  \centering
  \setlength{\abovecaptionskip}{3pt}
  \setlength{\belowcaptionskip}{3pt}
  \includegraphics[width=\linewidth]{figures/variants_scatter.pdf}
  \caption{\textbf{Accuracy and cost move together, and one instantiation holds the corner on both levels.} Solve rate against mean turns to termination for every instantiation of the bank (Claude Sonnet, training seeds); colour is the instantiation, shape is the level. Cheap and accurate is the shaded upper left, and Off2On Evolving, written simply as \textsc{HExA}, is its only occupant on either level; arrows run from each level's \textsc{Zero-shot} floor to its \textsc{HExA} point. The remaining variants cluster in the middle and change order between levels. Failures count at the $25$-turn cap; the $x$ axis is compressed below $10$ turns. Solve rates match Table~\ref{tab:variants_compact}.}
  \label{fig:training_curves}
  \label{fig:catapult_var_cum_accuracy}
  \label{fig:ptp_cum_accuracy}
\end{wrapfigure}
As Table~\ref{tab:variants_compact} shows, Off2On reaches $84.0\%$ and $68.0\%$ on
\texttt{catapult} and \texttt{pass\_the\_parcel} versus $44.0\%$ and $58.0\%$ for
a pure Online start. The gap is sharpest on \texttt{catapult}, where a cold start
wastes its early rounds rediscovering the level's basic dynamics, an advantage
that shrinks once enough online experimentation has been done. The update rule
matters on both levels: evolving the existing bank with each round's new
trajectories beats rebuilding it from the current rollouts alone, $84.0\%$ vs
$56.0\%$ on \texttt{catapult} and $68.0\%$ vs $48.0\%$ on
\texttt{pass\_the\_parcel}. Round-$n$ trajectories are generated while the actor
is conditioned on $\mathcal{G}_n=\textsc{Retriever}(\mathcal{K}_{n-1},\ell,M,N)$,
so they already reflect the previous round's skills; the evolutionary update can
then refine an earlier rule, find its boundary conditions, or replace it when
later evidence contradicts it, whereas rebuilding from scratch discards what has
accumulated and amplifies overfitting to the instances seen so far.
Figure~\ref{fig:training_curves} plots accuracy against cost: the
configurations that solve more also finish sooner.


\emph{How do reward labels help learning via experimentation?} We run
\textsc{HExA} with and without the reward labels on the skill bank. In the
ablation without them, every success and failure trajectory, and every skill
distilled out of them, is treated equally, and the LLM evolver implicitly updates
the bank using its existing knowledge rather than environment feedback. Removing
the labels costs accuracy on every level we test
(details in Figure~\ref{fig:reward_ablation}, Table~\ref{tab:reward_ablation_main}): on
\texttt{catapult} the reward-free variant drops Claude Sonnet from
$78.0 \pm 10.7\%$ to $51.0 \pm 10.1\%$, and on Qwen-2.5-7B it reaches
$64.0 \pm 1.7\%$ versus $72.0 \pm 5.2\%$ with rewards on
\texttt{down\_to\_earth} and $20.0 \pm 2.7\%$ versus $42.0 \pm 3.3\%$ on
\texttt{two\_body\_problem}. It also costs efficiency: the
reward-free bank needs $15.8$ iterations per seed on \texttt{catapult} against
$13.3$ with labels, $14.6$ against $12.6$ on \texttt{down\_to\_earth} and $22.2$
against $17.7$ on \texttt{two\_body\_problem},
so the labelled bank solves more seeds with fewer interactions. The reward labels
thus provide environment-grounded feedback from the actor's own exploration that
helps assign credit for effective and efficient skill acquisition, and better
guides the evolver in composing, retaining or pruning skills.




\subsection{Frozen-bank content and ranking ablations}
\label{app:bank-content}

\paragraph{Setup.} Because HExA's skill bank is injected as a textual prefix,
any improvement could in principle be attributed to prompt length, in-context
formatting, or generic priming toward physics reasoning rather than to the
specific knowledge the evolver distilled. We isolate this with frozen banks---no
evolution during evaluation---under four content conditions and four ranking
conditions Figure~\ref{fig:bank_ablation_full} and Table~\ref{tab:interphyre_ablation}.

\begin{figure}[H]
  \centering
  \includegraphics[width=1\linewidth]{figures/bank_ablation.pdf}
  \caption{%
    \textbf{Frozen-bank content and ranking ablations, full results.}
    Held-out solve rate (\%) on 50 unseen seeds of \texttt{two\_body\_problem}
    and \texttt{down\_to\_earth} with Qwen-2.5-7B and a frozen skill bank;
    points are means over 3 independent runs and bars denote $\pm 1$ s.d.
    The dashed line marks \textsc{ReAct} with an empty bank
    ($\mathcal{K} = \varnothing$), the shaded orange region marks performance
    worse than injecting nothing, and the blue band marks $\pm 1$ s.d.\ around
    the full-bank reference. The \emph{injected context} column reports the
    character count of the retrieved prefix, so each condition's accuracy can
    be read against the amount of text it adds.
    \emph{Top:} which components of the bank are injected---full bank,
    strategy skills only, mistake records only, or a length-matched bank
    evolved on a different level.
    \emph{Bottom:} whether the evolver's reward-derived confidence ranking
    carries information---all skills retained, the two lowest-confidence
    skills removed, the two highest removed, or confidences randomly permuted
    while retaining all content.}
  \label{fig:bank_ablation_full}
\end{figure}

\paragraph{Strategy skills and mistake records are not interchangeable.}
Removing either component costs accuracy, but the two behave differently across
levels. Strategy skills alone retain most of the gain on both levels
($46.0\%$ and $71.4\%$). Mistake records alone are nearly sufficient on
\texttt{down\_to\_earth} ($74.8\%$ of a $76.9\%$ ceiling) yet collapse on
\texttt{two\_body\_problem} ($17.3\%$). We read this as a difference in failure
structure: on the easier level most failures are recurring, locally correctable
errors that a record of past mistakes prevents directly, whereas the harder
level requires a positive multi-step strategy---bisection over a contact
parameter, in the worked example of Appendix~\ref{app:worked-example}---that
descriptions of what went wrong do not supply. This supports maintaining both
skill types rather than a single undifferentiated memory.

\paragraph{The evolver's confidences are informative, not decorative.}
On \texttt{down\_to\_earth}, removing the two highest-confidence skills costs
$11.4$ points ($76.7\% \rightarrow 65.3\%$), whereas removing the two lowest
leaves performance unchanged ($76.7\%$) despite halving the injected context
from $0.9$k to $0.5$k characters: the ranking identifies which entries carry the
task, and the low-ranked tail is close to free to discard. Permuting confidences
while retaining all content costs $6.0$ points on \texttt{down\_to\_earth}
($76.7\% \rightarrow 70.7\%$), indicating that retrieval order matters beyond
mere inclusion, though on \texttt{two\_body\_problem} the same manipulation lies
within run-to-run variance ($50.0\% \rightarrow 48.7\%$). We therefore treat
ranking quality as a secondary rather than primary driver of performance.

\paragraph{Relevance, not volume: the wrong-level control.}
We replace the bank with one evolved on a different \textsc{Interphyre} level,
matched in length and indistinguishable in surface form: fluent, well-structured
physics guidance with the same schema of titles, principles and applicability
conditions. On \texttt{two\_body\_problem} this reduces solve rate from $50.0\%$
to $9.3\%$, below the $12.0\%$ empty-bank \textsc{ReAct} baseline, while
injecting $2.9$k characters against the full bank's $4.0$k; the same ordering
holds on \texttt{down\_to\_earth} ($76.9\% \rightarrow 27.9\%$). Injecting
plausible but misapplied procedural knowledge is therefore actively harmful
relative to injecting nothing, which rules out length and priming explanations:
a longer prompt that is wrong about the task is worse than no prompt at all. We
attribute this to misdirected exploration---the actor commits early to a
strategy whose applicability condition does not in fact hold, and spends its
$25$-turn budget refining the wrong hypothesis rather than forming a new one.
This is also why cross-level transfer (Section~\ref{sec:transfer}) requires the
evolver's de-binding and re-grounding step rather than direct reuse of a source
bank.

\paragraph{Summary.} These ablations locate HExA's gain in task-relevant
distilled content and its reward-derived prioritization, not in context length.
Both skill types are load-bearing, their relative importance tracks the failure
structure of the level, and the bank's value concentrates in a small number of
high-confidence strategies.

\input{tables/ablations_merged}
