# Supplementary material for: Hierarchical Experimentalist Agents
Source: arXiv:2606.29315 source file (2026-10-09)
Supplement: Supplementary file 4 [file app_results_old.tex]

\section{Full results}
\label{app:results}

This appendix holds the detailed counterparts of the five compressed tables in
Section~\ref{sec:results}: per-episode metrics, token ranges, iteration counts,
competing published numbers and the full significance blocks.

% =====================================================================
\subsection{\textsc{InterPhyre}}
\label{app:results:interphyre}

The \textsc{Zero-shot} base rate on every level is in the main body
(Table~\ref{tab:direct_baseline_results_main}).
Table~\ref{tab:catapult_cost} gives the cost accounting on the two hard levels
with Claude Sonnet, and Table~\ref{tab:interphyre_qwen_full} the open-weight
head-to-head with per-replicate standard deviations. These are the
sources for the corresponding columns of Table~\ref{tab:interphyre}.

We also ran GPT-OSS-120B on \texttt{catapult}, where \textsc{HExA} lifts it from
$0.0\%$ under \textsc{ReAct} to $54.0\%$. That run predates the fixed split and
is scored on the pooled seed set, with the bank not yet distilled on the seed
being attempted, so it is not paired with the arms in
Table~\ref{tab:interphyre} and we keep it out of that table.

\input{tables/catapult_main}
\input{tables/interphyre_qwen}

\begin{figure}[t]
  \centering
  \begin{minipage}[t]{0.49\linewidth}
    \centering
    \includegraphics[width=\linewidth]{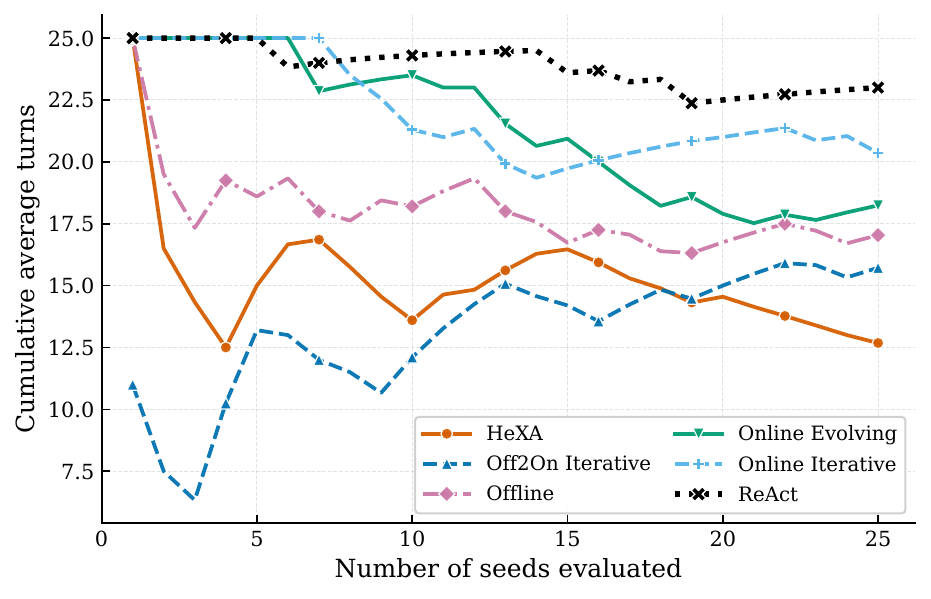}
    \subcaption{Catapult}
    \label{fig:catapult_var_cum_iter}
  \end{minipage}\hfill
  \begin{minipage}[t]{0.49\linewidth}
    \centering
    \includegraphics[width=\linewidth]{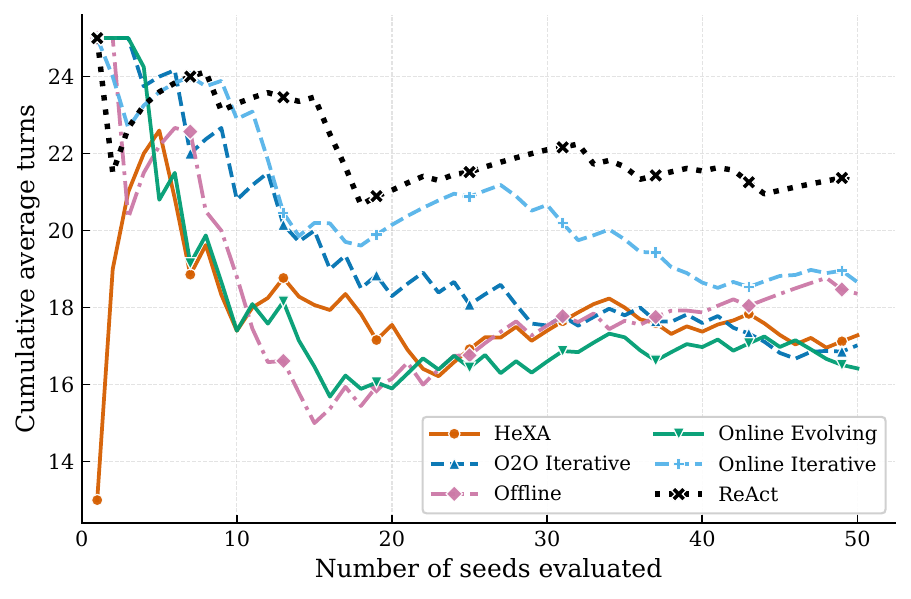}
    \subcaption{Pass the Parcel}
    \label{fig:ptp_cum_iter}
  \end{minipage}
  \caption{%
    \textbf{Cumulative average turns per seed}, Claude Sonnet; lower is more
    efficient. Off2On Evolving converges to the lowest cost per seed on both
    levels, while the iterative and pure-online variants stay higher, so the gain
    comes from guiding search with accumulated experience rather than from
    spending more computation per instance. The cumulative curves stay separated
    across the whole seed sweep, so the ranking is not an artifact of a few lucky
    seeds. Companion to Figure~\ref{fig:training_curves}.}
  \label{fig:cum_iter_both}
\end{figure}

\begin{figure}[t]
\centering
\setlength{\tabcolsep}{1.2pt}
\renewcommand{\arraystretch}{0.85}
{\footnotesize\itshape \textsc{ReAct} (25 iterations, FAILURE)}\\[1pt]
\begin{tabular}{@{}ccccccc@{}}
  \includegraphics[width=0.135\linewidth]{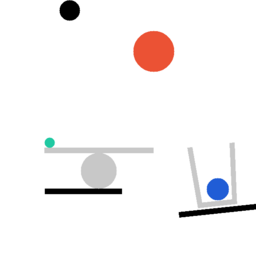} &
  \includegraphics[width=0.135\linewidth]{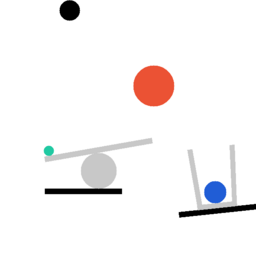} &
  \includegraphics[width=0.135\linewidth]{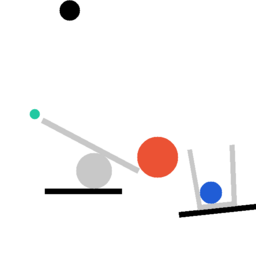} &
  \includegraphics[width=0.135\linewidth]{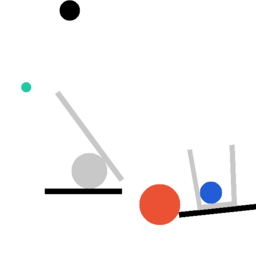} &
  \includegraphics[width=0.135\linewidth]{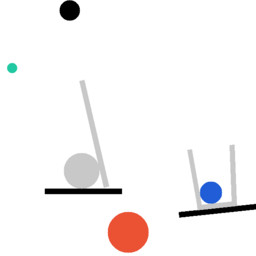} &
  \includegraphics[width=0.135\linewidth]{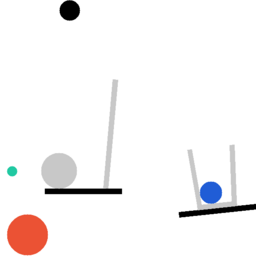} &
  \includegraphics[width=0.135\linewidth]{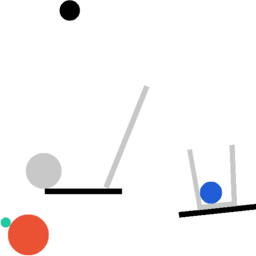} \\
\end{tabular}\\[2pt]
{\footnotesize\itshape \textsc{HExA} (6 iterations, SUCCESS)}\\[1pt]
\begin{tabular}{@{}ccccccc@{}}
  \includegraphics[width=0.135\linewidth]{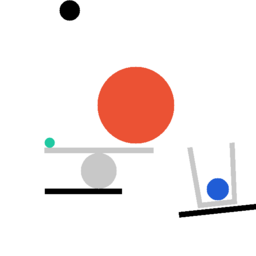} &
  \includegraphics[width=0.135\linewidth]{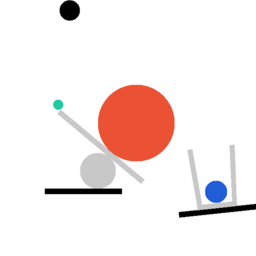} &
  \includegraphics[width=0.135\linewidth]{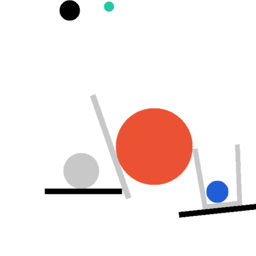} &
  \includegraphics[width=0.135\linewidth]{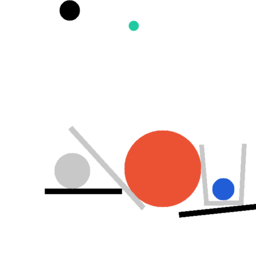} &
  \includegraphics[width=0.135\linewidth]{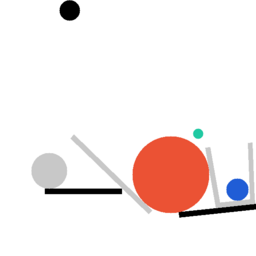} &
  \includegraphics[width=0.135\linewidth]{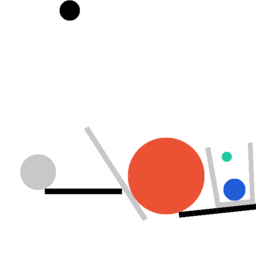} &
  \includegraphics[width=0.135\linewidth]{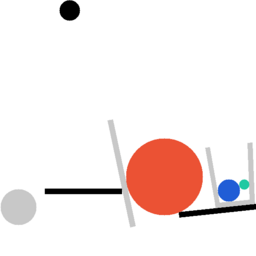} \\
\end{tabular}
\caption{%
\textbf{How the evolved bank guides the agent on a held-out \texttt{catapult}
seed.} Top: \textsc{ReAct}, with no cross-episode memory, exhausts its
25-iteration budget on ineffective placements. Bottom: \textsc{HExA} opens with
the bank's learned default, reads the resulting failure through the bank's
diagnosis rather than as a reason to keep tuning the same parameter, applies the
corrective rule, and succeeds in six interaction iterations. Frames are sampled
from the final simulations; full prompts, bank entries and trajectories are in
Appendix~\ref{app:trajectories:bank}.}
\utsav{These frames are still rendered from seed 45. They have to be re-made for
seed 64, to match the skill-bank box in the method section and the transcripts in
Appendix~\ref{app:trajectories}. The caption above is already seed-agnostic, so
only the images and the iteration counts need swapping.}
\label{fig:catapult45_simframes}
\end{figure}

\input{tables/baseline_results}

% =====================================================================
\subsection{Interactive games}
\label{app:results:games}

Table~\ref{tab:orbit_memory} is the full head-to-head on Mastermind and Maze:
three task/actor blocks, each arm playing an identical held-out pool, with
first-episode, last-episode and \texttt{any}-episode success, the injected token
budget, and a two-sided paired sign test on episode-3 outcomes against that
block's no-memory arm. Table~\ref{tab:orbit_transfer_full} gives the per-episode
breakdown of the cross-task transfer arms summarised in
Table~\ref{tab:transfer}.

\input{tables/orbit_memory_headtohead}
\subsection{Reasoning and planning}
\label{app:results:reasoning}

Table~\ref{tab:reasoning} gives the per-task head-to-head on the four reasoning
and planning tasks. Every arm is our own run on our provider at the same rollout
budget as \textsc{HExA}, so all rows are paired on identical items; the MemRL
runs at this budget are still in progress.

\input{tables/core_headtohead}

% =====================================================================
\subsection{\textsc{DiscoverPhysics}}
\label{app:results:discovery}

Table~\ref{tab:discovery} gives explanation score, benchmark reward and pass-rate
at both gates for all three worlds, with exact paired tests on the same 15 seeds.

\input{tables/discovery}

% =====================================================================
\subsection{Transfer}
\label{app:results:transfer}

Table~\ref{tab:cross_level_full} reports the source-bank and synthesised-bank
sizes for cross-level transfer within \textsc{InterPhyre}, and
Table~\ref{tab:orbit_transfer_full} the per-episode breakdown for cross-task
transfer on Mastermind.

\input{tables/cross_level_transfer}
\input{tables/orbit_transfer}

% =====================================================================
\subsection{In-context accumulation against gradient-based RL}
\label{app:results:grpo}

To situate \textsc{HExA} in the broader RL landscape, we train the same
Qwen-2.5-3B model on the same two levels with Group Relative Policy Optimization
(GRPO)~\citep{shao2024deepseekmath}, using batch size $1$, $n{=}4$ rollouts per
step, and a binary $\{0, 1\}$ reward from the environment. With 50 training seeds
and batch size $1$, one epoch of GRPO corresponds to 50 gradient updates --- the
same number of unique puzzle instances seen by \textsc{HExA} in a single pass.
Figure~\ref{fig:grpo_comparison} shows validation accuracy across 6 epochs for two
variants: GRPO, and GRPO with a previously evolved skill bank baked into the
prompt at data-generation time.

\input{figures/grpo_comparision_figure}

At the matched sample budget (50 unique seeds, vertical dashed line), GRPO
without skills reaches $20\%$ on \texttt{down\_to\_earth} and $6\%$ on
\texttt{two\_body\_problem}, against \textsc{HExA}'s $23.3\%$ and $12.0\%$. This
gap is consistent with the established finding that in-context methods are more
sample-efficient in new domains: skills distilled from early trajectories are
immediately available to subsequent episodes via context injection, whereas GRPO
must accumulate gradient signal over many rollouts before the policy weights
encode the same knowledge.

Given sufficient training, however, GRPO's exact environment reward eventually
dominates: \texttt{down\_to\_earth} reaches $100\%$ by epoch~5 (GRPO) and epoch~6
(GRPO with skills), while \texttt{two\_body\_problem} peaks at $56\%$ and plateaus
around $40$--$50\%$ for GRPO and converges to $100\%$ by epoch~4 with skills. The
skilled variant additionally exhibits a pronounced epoch-1 dip ($6\%$ on
\texttt{down\_to\_earth}, $0\%$ on \texttt{two\_body\_problem}) before recovering,
consistent with the model needing several epochs to re-adapt its generation format
to the longer skill-augmented prompt (${\sim}2200$ vs.\ ${\sim}1400$ tokens)
before it can leverage the injected skills. In-context skill evolution is
therefore the preferred approach when the sample and interaction budget is small,
while gradient-based RL with an exact reward remains a strong option to bootstrap
further after an in-context warm start.

\input{tables/ICMSRL_results}
\input{tables/ICMSRL_catapult_variants}
